# Supplementary material for: Strong coupling of virtual negative states in the Kapitza-Dirac effect
Source: arXiv:2601.07157 ancillary file (2026-05-19)
Supplement: Supplementary file 1 [file supplemental_material.pdf]

# Strong coupling of virtual negative states in the Kapitza-Dirac effect
# Supplemental Material

Qianlong Wang,[1] Sven Ahrens,[1,*] and Baifei Shen[1,†]

[1] *Department of Physics, Shanghai Normal University, Shanghai 200234, China*

(Dated: January 12, 2026)

## I. THE RELATIVISTIC PONDEROMOTIVE POTENTIAL IN THE KAPITZA-DIRAC EFFECT

The electric field and magnetic field are given by

$$\boldsymbol{E}(\boldsymbol{x},t) = -\frac{1}{c}\frac{\partial \boldsymbol{A}}{\partial t} = -A_0 k_L \cos(k_L x)\cos(\omega t)\boldsymbol{e}_3 \tag{1a}$$

$$\boldsymbol{B}(\boldsymbol{x},t) = \boldsymbol{\nabla}\times\boldsymbol{A} = A_0 k_L \sin(k_L x)\sin(\omega t)\boldsymbol{e}_2 \,. \tag{1b}$$

In the following calculation we assume that except the original particle position $\boldsymbol{x}$ and momentum $\boldsymbol{p}$ no further additional integration constants arise when computing the anti-derivatives. This corresponds to the assumption case that the electron is adiabatically entering and exiting the laser field. We further introduce the oscillation amplitudes

$$\delta\boldsymbol{x} = \tilde{\boldsymbol{x}} - \boldsymbol{x}\,, \qquad \delta\boldsymbol{p} = \tilde{\boldsymbol{p}} - \boldsymbol{p}\,. \tag{2}$$

The initial electron momentum is set to $\boldsymbol{p} = p_3\boldsymbol{e}_3$. The relativistic Lorentz force can be written as

$$\boldsymbol{F} = \frac{d\boldsymbol{p}}{dt} = e\left[\boldsymbol{E}(\boldsymbol{x},t) + \frac{\boldsymbol{p}}{m\gamma(\boldsymbol{p})}\times\boldsymbol{B}(\boldsymbol{x},t)\right]\,, \tag{3}$$

where the inverse of the relativistic gamma factor can be Taylor expanded as

$$\gamma^{-1}(\boldsymbol{p}) = \sqrt{1+\frac{\boldsymbol{p}}{mc^2}} \approx 1 - \frac{p_3^2}{2m^2c^2}\,. \tag{4}$$

We then obtain the modified particle momentum $\tilde{\boldsymbol{p}}$ from integrating Eq. (3), which reads

$$\tilde{\boldsymbol{p}} = \frac{eA_0p_3}{mc^2}\sin(k_L x)\cos(\omega t)\boldsymbol{e}_1 + \left[p_3 - \frac{eA_0}{c}\cos(k_L x)\sin(\omega t)\right]\boldsymbol{e}_3\,, \tag{5}$$

where we have omitted a term of third power in the momentum $p_3$. The Taylor expansion of the gamma factor for this modified momentum is

$$\gamma^{-1}(\tilde{\boldsymbol{p}}) \approx 1 - \frac{\tilde{p}_1^2}{2m^2c^2} - \frac{\tilde{p}_3^2}{2m^2c^2} + \frac{3\tilde{p}_1^2\tilde{p}_3^2}{4m^4c^4} \tag{6}$$

and expands as

$$\gamma^{-1}(\tilde{\boldsymbol{p}}) = 1 - \frac{e^2A_0^2p_3^2}{2m^4c^6}\sin^2(k_L x)\cos^2(\omega t) - \frac{p_3^2}{2m^2c^2} - \frac{e^2A_0^2}{2m^2c^4}\cos^2(k_L x)\sin^2(\omega t) + \frac{eA_0p_3}{m^2c^3}\cos(k_L x)\sin(\omega t) \tag{7}$$

on substituting $\tilde{p}_1$ and $\tilde{p}_3$ of the modified momentum (5).

* ahrens@shnu.edu.cn
† bfshen@shnu.edu.cn

The updated position in $x$-direction is

$$\begin{aligned}\tilde{x} =& \int \left(1 - \frac{\tilde{p}_1^2}{2m^2c^2} - \frac{\tilde{p}_3^2}{2m^2c^2}\right) \frac{\tilde{p}_1}{m} dt' \\ =& \int \left(1 - \frac{e^2A_0^2p_3^2}{2m^4c^6}\sin^2(k_Lx)\cos^2(\omega t') - \frac{p_3^2}{2m^2c^2} - \frac{e^2A_0^2}{2m^2c^4}\cos^2(k_Lx)\sin^2(\omega t') + \frac{eA_0p_3}{m^2c^3}\cos(k_Lx)\sin(\omega t')\right) \\ &\times \frac{eA_0p_3}{m^2c^2}\sin(k_Lx)\cos(\omega t')\ dt' \\ =& \int \left(\frac{eA_0p_3}{m^2c^2}\sin(k_Lx)\cos(\omega t') - \frac{e^3A_0^3p_3^3}{2m^6c^8}\sin^3(k_Lx)\cos^3(\omega t') - \frac{eA_0p_3^3}{2m^4c^4}\sin(k_Lx)\cos(\omega t') \right. \\ &\left. - \frac{e^3A_0^3p_3}{2m^4c^6}\sin(k_Lx)\cos^2(k_Lx)\sin^2(\omega t')\cos(\omega t') + \frac{e^2A_0^2p_3^2}{m^4c^5}\cos(k_Lx)\sin(k_Lx)\cos(\omega t')\sin(\omega t')\right) dt' \,. \end{aligned} \tag{8}$$

If we neglect the higher order terms which are associated with $p_3^3$ and $A_0^3$ and integrate (8), we obtain

$$\tilde{x} = \frac{eA_0p_3}{m^2c^2\omega}\sin(k_Lx)\sin(\omega t) + \frac{e^2A_0^2p_3^2}{2m^4c^5\omega}\cos(k_Lx)\sin(k_Lx)\sin^2(\omega t) + x\,, \tag{9}$$

which means that the explicit expression for the oscillation position along the $x$-direction is

$$\delta x = \frac{eA_0p_3}{m^2c^2\omega}\sin(k_Lx)\sin(\omega t) + \frac{e^2A_0^2p_3^2}{2m^4c^5\omega}\cos(k_Lx)\sin(k_Lx)\sin^2(\omega t)\,. \tag{10}$$

At these updated positions, the fields can be approximated as

$$\tilde{\boldsymbol{E}} = \boldsymbol{E}(\tilde{\boldsymbol{x}}, t) \approx \boldsymbol{E}(\boldsymbol{x}, t) + \delta\boldsymbol{E} \tag{11a}$$

$$\tilde{\boldsymbol{B}} = \boldsymbol{B}(\tilde{\boldsymbol{x}}, t) \approx \boldsymbol{B}(\boldsymbol{x}, t) + \delta\boldsymbol{B}\,. \tag{11b}$$

The small quantities $\delta\boldsymbol{E}$ and $\delta\boldsymbol{B}$ are the terms of the first order Taylor expansion, which contain the field derivatives

$$\frac{\partial}{\partial x}\boldsymbol{E}(\boldsymbol{x}, t) = A_0k_L^2\sin(k_Lx)\cos(\omega t)\boldsymbol{e}_3 \tag{12a}$$

$$\frac{\partial}{\partial x}\boldsymbol{B}(\boldsymbol{x}, t) = A_0k_L^2\cos(k_Lx)\sin(\omega t)\boldsymbol{e}_2\,. \tag{12b}$$

Thus, combining (12) with (10) yields the first order Taylor expansion contributions

$$\delta\boldsymbol{E} = \delta x\frac{\partial}{\partial x}\boldsymbol{E} = \frac{eA_0^2k_Lp_3}{m^2c^3}\sin^2(k_Lx)\sin(\omega t)\cos(\omega t)\boldsymbol{e}_3, \tag{13a}$$

$$\delta\boldsymbol{B} = \delta x\frac{\partial}{\partial x}\boldsymbol{B} = \frac{eA_0^2k_Lp_3}{m^2c^3}\sin(k_Lx)\cos(k_Lx)\sin^2(\omega t)\boldsymbol{e}_2\,, \tag{13b}$$

where we again neglect the higher order terms, which are associated with $A_0^3$.

The updated fields $\tilde{\boldsymbol{E}}$ and $\tilde{\boldsymbol{B}}$ at the updated position $\tilde{\boldsymbol{x}}$ and momentum $\tilde{\boldsymbol{p}}$ result in the modified relativistic force

$$\tilde{\boldsymbol{F}} \approx e\left[(\boldsymbol{E} + \delta\boldsymbol{E}) + \frac{\tilde{\boldsymbol{p}}}{\gamma(\tilde{\boldsymbol{p}})mc} \times (\boldsymbol{B} + \delta\boldsymbol{B})\right]\,. \tag{14}$$

We want to compute the average of this modified relativistic force and first expand

$$\begin{aligned}\frac{\tilde{\boldsymbol{p}}}{\gamma(\tilde{\boldsymbol{p}})} =& \left\{\frac{eA_0p_3}{mc^2}\sin(k_Lx)\cos(\omega t)\boldsymbol{e}_1 + \left[p_3 - \frac{eA_0}{c}\cos(k_Lx)\sin(\omega t)\right]\boldsymbol{e}_3\right\} \\ &\times\left[1 - \frac{e^2A_0^2p_3^2}{2m^4c^6}\sin^2(k_Lx)\cos^2(\omega t) - \frac{p_3^2}{2m^2c^2} - \frac{e^2A_0^2}{2m^2c^4}\cos^2(k_Lx)\sin^2(\omega t) + \frac{eA_0p_3}{m^2c^3}\cos(k_Lx)\sin(\omega t)\right]\,, \end{aligned} \tag{15}$$

where terms like $p_3^3$ and $A_0^3$, which are larger than second order in $p_3$ and $A_0$, are neglected. For ease of notion, we write

$$\frac{\tilde{\boldsymbol{p}}}{\gamma(\tilde{\boldsymbol{p}})} = \mathcal{A} + \mathcal{B} + \mathcal{C} + \mathcal{D} + \mathcal{F} + \mathcal{G} \tag{16}$$

by introducing the expressions

$$\mathcal{A} = \frac{eA_0 p_3}{mc^2}\sin(k_L x)\cos(\omega t)\boldsymbol{e}_1, \tag{17a}$$

$$\mathcal{B} = \frac{e^2 A_0^2 p_3^2}{m^3 c^5}\sin(k_L x)\cos(k_L x)\sin(\omega t)\cos(\omega t)\boldsymbol{e}_1, \tag{17b}$$

$$\mathcal{C} = p_3 \boldsymbol{e}_3, \tag{17c}$$

$$\mathcal{D} = -\frac{3e^2 A_0^2 p_3}{2m^2 c^4}\cos^2(k_L x)\sin^2(\omega t)\boldsymbol{e}_3, \tag{17d}$$

$$\mathcal{F} = \frac{3eA_0 p_3^2}{2m^2 c^3}\cos(k_L x)\sin(\omega t)\boldsymbol{e}_3, \tag{17e}$$

$$\mathcal{G} = -\frac{eA_0}{c}\cos(k_L x)\sin(\omega t)\boldsymbol{e}_3. \tag{17f}$$

$$\tag{17g}$$

The relativistic ponderomotive force is associated with the average of the force (14) over one laser cycle

$$\langle \tilde{\boldsymbol{F}} \rangle = \frac{\omega}{2\pi}\int_{t_0}^{t_0+\frac{2\pi}{\omega}} \tilde{\boldsymbol{F}} dt\,. \tag{18}$$

The evaluation of the expression $\langle e(\boldsymbol{E}+\delta\boldsymbol{E})\rangle$ vanishes.

$$\langle e(\boldsymbol{E}+\delta\boldsymbol{E})\rangle = \frac{\omega}{2\pi}\int_{t_0}^{t_0+\frac{2\pi}{\omega}} e\Big[-A_0 k_L\cos(k_L x)\cos(\omega t') + \frac{eA_0^2 k_L p_3}{m^2c^3}\sin^2(k_L x)\sin(\omega t')\cos(\omega t')\Big]\boldsymbol{e}_3\, dt' = 0 \tag{19}$$

All integration results of the $\langle \frac{\tilde{\boldsymbol{p}}}{\gamma(\tilde{\boldsymbol{p}})}\times(\boldsymbol{B}+\delta\boldsymbol{B})\rangle$ expression expand as

$$\langle \mathcal{A}\times\boldsymbol{B}\rangle = \frac{\omega}{2\pi}\int_{t_0}^{t_0+\frac{2\pi}{\omega}} \frac{eA_0^2 k_L p_3}{mc^2}\sin^2(k_L x)\sin(\omega t')\cos(\omega t')\boldsymbol{e}_3\, dt' = \boldsymbol{0} \tag{20a}$$

$$\langle \mathcal{B}\times\boldsymbol{B}\rangle = \frac{\omega}{2\pi}\int_{t_0}^{t_0+\frac{2\pi}{\omega}} \frac{e^2 A_0^3 k_L p_3^2}{m^3c^5}\sin^2(k_L x)\cos(k_L x)\sin^2(\omega t')\cos(\omega t')\boldsymbol{e}_3\, dt' = \boldsymbol{0} \tag{20b}$$

$$\langle \mathcal{C}\times\boldsymbol{B}\rangle = \frac{\omega}{2\pi}\int_{t_0}^{t_0+\frac{2\pi}{\omega}} -A_0 k_L p_3\sin(k_L x)\sin(\omega t')\boldsymbol{e}_1\, dt' = \boldsymbol{0} \tag{20c}$$

$$\langle \mathcal{D}\times\boldsymbol{B}\rangle = \frac{\omega}{2\pi}\int_{t_0}^{t_0+\frac{2\pi}{\omega}} \frac{3e^2 A_0^3 k_L p_3}{2m^2c^4}\sin(k_L x)\cos^2(k_L x)\sin^3(\omega t')\boldsymbol{e}_1\, dt' = \boldsymbol{0} \tag{20d}$$

$$\langle \mathcal{F}\times\boldsymbol{B}\rangle = \frac{\omega}{2\pi}\int_{t_0}^{t_0+\frac{2\pi}{\omega}} -\frac{3eA_0^2 k_L p_3^2}{2m^2c^3}\sin(k_L x)\cos(k_L x)\sin^2(\omega t')\boldsymbol{e}_1\, dt' \neq \boldsymbol{0} \tag{20e}$$

$$\langle \mathcal{G}\times\boldsymbol{B}\rangle = \frac{\omega}{2\pi}\int_{t_0}^{t_0+\frac{2\pi}{\omega}} \frac{eA_0^2 k_L}{c}\sin(k_L x)\cos(k_L x)\sin^2(\omega t')\boldsymbol{e}_1\, dt' \neq \boldsymbol{0} \tag{20f}$$

$$\langle \mathcal{A}\times\delta\boldsymbol{B}\rangle = \frac{\omega}{2\pi}\int_{t_0}^{t_0+\frac{2\pi}{\omega}} \frac{e^2 A_0^3 k_L p_3^2}{m^3c^5}\sin^2(k_L x)\cos(k_L x)\sin^2(\omega t')\cos(\omega t')\boldsymbol{e}_3\, dt' = \boldsymbol{0} \tag{20g}$$

$$\langle \mathcal{B}\times\delta\boldsymbol{B}\rangle = \frac{\omega}{2\pi}\int_{t_0}^{t_0+\frac{2\pi}{\omega}} \frac{e^3 A_0^4 k_L p_3^3}{m^5c^8}\sin^2(k_L x)\cos^2(k_L x)\sin^3(\omega t')\cos(\omega t')\boldsymbol{e}_3\, dt' = \boldsymbol{0} \tag{20h}$$

$$\langle \mathcal{C}\times\delta\boldsymbol{B}\rangle = \frac{\omega}{2\pi}\int_{t_0}^{t_0+\frac{2\pi}{\omega}} -\frac{eA_0^2 k_L p_3^2}{m^2c^3}\sin(k_L x)\cos(k_L x)\sin^2(\omega t')\boldsymbol{e}_1\, dt' \neq \boldsymbol{0} \tag{20i}$$

$$\langle \mathcal{D}\times\delta\boldsymbol{B}\rangle = \frac{\omega}{2\pi}\int_{t_0}^{t_0+\frac{2\pi}{\omega}} \frac{3e^3 A_0^4 k_L p_3^2}{2m^4c^7}\sin(k_L x)\cos^3(k_L x)\sin^4(\omega t')\boldsymbol{e}_1\, dt' \neq \boldsymbol{0} \tag{20j}$$

$$\langle \mathcal{F}\times\delta\boldsymbol{B}\rangle = \frac{\omega}{2\pi}\int_{t_0}^{t_0+\frac{2\pi}{\omega}} -\frac{3e^2 A_0^3 k_L p_3^3}{2m^4c^6}\sin(k_L x)\cos^2(k_L x)\sin^3(\omega t')\boldsymbol{e}_1\, dt' = \boldsymbol{0} \tag{20k}$$

$$\langle \mathcal{G}\times\delta\boldsymbol{B}\rangle = \frac{\omega}{2\pi}\int_{t_0}^{t_0+\frac{2\pi}{\omega}} \frac{e^2 A_0^3 k_L p_3}{m^2c^4}\sin(k_L x)\cos^2(k_L x)\sin^3(\omega t')\boldsymbol{e}_1\, dt' = \boldsymbol{0}\,. \tag{20l}$$

The only non-vanishing terms in Eq. (20) are Eqs. (20e), (20f), (20i) and (20j). We will neglect Eq. (20j), because it is of order $A_0^4$.

After removing the vanishing terms and higher order terms, the time-averaged modified relativistic force is given by

$$\begin{aligned}\langle\tilde{\boldsymbol{F}}\rangle &= \frac{e}{mc}\left\langle\frac{\tilde{\boldsymbol{p}}}{\gamma(\tilde{\boldsymbol{p}})}\times(\boldsymbol{B}+\delta\boldsymbol{B})\right\rangle = \frac{e}{mc}\left(\langle\mathcal{G}\times\boldsymbol{B}\rangle+\langle\mathcal{F}\times\boldsymbol{B}\rangle+\langle\mathcal{C}\times\delta\boldsymbol{B}\rangle\right)\\ &= \frac{\omega e}{2\pi mc}\int_{t_0}^{t_0+\frac{2\pi}{\omega}}\left[\frac{eA_0^2k_L}{c}\left(1-\frac{5p_3^2}{2m^2c^2}\right)\sin(k_Lx)\cos(k_Lx)\sin^2(\omega t)\right]\boldsymbol{e}_1dt\\ &= \left[\frac{e^2A_0^2k_L}{2mc^2}\left(1-\frac{5p_3^2}{2m^2c^2}\right)\sin(k_Lx)\cos(k_Lx)\right]\boldsymbol{e}_1. \end{aligned} \tag{21}$$

The ponderomotive potential is obtained by integrating the time-averaged modified relativistic force (21) along the direction of the only non-trivial spacial dependence (ie. along the laser propagation direction) is

$$V_{\text{pond}} = -\int\langle\tilde{\boldsymbol{F}}\rangle\cdot\boldsymbol{e}_1dx = \frac{e^2A_0^2}{4mc^2}\left(1-\frac{5p_3^2}{2m^2c^2}\right)\cos^2(k_Lx)\,. \tag{22}$$
